# Supplementary material for: Provably efficient RL with Rich Observations via Latent State Decoding
Source: arXiv:1901.09018 source file (2021-09-09)
Supplement: Supplementary file 1 [file additional_exp.tex]

Here we study the output of our algorithm to test whether it matches the theory.
In our experiment, we test $d = 5$ and $H=10$.
We use linear function class and set $N_{exp} = N_{id} = 1000$.
When $h \ge 2$, for $s_2$ there are 3 ways of getting there, and for $s_1$ there is only one way, so the underlying true linear regressor is \begin{align*}
	B = \begin{pmatrix}
	0.1 & 0 & 0 & \ldots& 0 \\
	0 & 1/30 & 0 &\ldots & 0 \\
	0 & 1/30 & 0 &\ldots & 0 \\
	0 & 1/30 & 0 &\ldots & 0 \\ 
	\end{pmatrix}.
\end{align*} 
To see this, note if  $x \sim E(s_1)$, \begin{align*}
	Bx = \begin{pmatrix}
	0.1 & 0 & 0 &  \ldots& 0 \\
	0 & 1/30 & 0 &\ldots & 0 \\
	0 & 1/30 & 0  &\ldots & 0 \\
	0 & 1/30 & 0  &\ldots & 0 \\ 
	\end{pmatrix} \begin{pmatrix}
	10\\
	0\\
	?\\
	...\\
	?
	\end{pmatrix} = \begin{pmatrix}
	1\\
	0 \\
	0\\
	0
	\end{pmatrix}
\end{align*} which is exactly $P(s,a|s_1)$.
Similarly if $x\sim E(s_2)$, we have \begin{align*}
Bx = \begin{pmatrix}
0.1 & 0 & 0 &  \ldots& 0 \\
0 & 1/30 & 0 &\ldots & 0 \\
0 & 1/30 & 0  &\ldots & 0 \\
0 & 1/30 & 0  &\ldots & 0 \\ 
\end{pmatrix} \begin{pmatrix}
0\\
10\\
?\\
...\\
?
\end{pmatrix} = \begin{pmatrix}
0\\
1/3 \\
1/3\\
1/3
\end{pmatrix}
\end{align*} which is $P(s,a|s_2)$.
We sampled some learned $\hat{g}_h$.

$\hat{g}_3$:\begin{verbatim}
0.0968    0.0008    0.0005    0.0002   -0.0000
-0.0004    0.0334    0.0013   -0.0223   -0.0056
-0.0008    0.0325    0.0119    0.0337    0.0287
0.0013    0.0338   -0.0141   -0.0106   -0.0248
\end{verbatim}

$\hat{g}_7$:\begin{verbatim}
0.0970   -0.0001   -0.0062    0.0029    0.0028
0.0000    0.0309   -0.0210    0.0183   -0.0203
0.0011    0.0358    0.0148   -0.0102    0.0078
0.0002    0.0330    0.0056   -0.0078    0.0100
\end{verbatim}

$\hat{g}_{10}$: \begin{verbatim}
0.0972    0.0003    0.0031    0.0005    0.0006
-0.0004    0.0353   -0.0153   -0.0110   -0.0040
-0.0000    0.0319    0.0189    0.0039    0.0180
-0.0008    0.0326   -0.0045    0.0059   -0.0158
\end{verbatim}

\simon{What other things should we show?}

\subsection{Stochastic Contextual Combination Lock}
\label{sec:stoc_comb_lock}
We next consider a hard stochastic problem, stochastic contextual combination lock.
There are two actions, $a$ and $b$.
There is only one state at $h=0$, $\states_0 = \left\{s_0\right\}$.
There are two states at $h=1$, $\states_1 = \left\{s_1,s_2\right\}$.
The transition rule at level $h=0$ is $P(\cdot|s_0,a) = \left[0.9,0.1\right]$ and $P(\cdot|s_1,a) = \left[0.1,0.9\right]$.

For $h \ge 2$, there are 3 states $\states_h = \left\{s_1,s_2,s_3\right\}$.
$s_3$ is the dead-end state, i.e., $P(\cdot|s_3,a) = P(\cdot|s_3,b) = [0,0,1]$.
The transition probability at $s_1$ is $P(\cdot|s_1,a) = [0.9,0.1,0]$  and $P(\cdot|s_1,b) = [0,0,1]$.
The transition probability at $s_2$ is $P(\cdot|s_2,a) = [0,0,1]$  and $P(\cdot|s_2,b) = [0.1,0.9,0]$.
At $s_1$, $a$ is the right action and at $s_2$, $b$ is the right action.
Therefore, we need to decode the state otherwise we cannot choose the right action.

We generate the context according the following rules.
If $s=s_1$, the first 3 coordinates are fixed $x_1 = 10$, $x_2 = 0$, $x_3=0$  and remaining ones are random $x_{4:d} \sim Bern(0.5)$, if $s=s_2$, the first 3 coordinates are fixed $x_1 = 0$, $x_2 = 10$, $x_3 = 10$  and remaining ones are random $x_{4:d} \sim Bern(0.5)$ and if $s=s_3$, the first 3 coordinates are fixed $x_1 = 0$, $x_2 = 0$, $x_3 = 10$  and remaining ones are random $x_{4:d} \sim Bern(0.5)$. 

\subsubsection{Study of Our Algorithm}
In our experiment, we test $d=5$, $H=10$.
We use linear function class and set $N_{exp} = 10000$, $N_{id}=100$, $N_{p}=10000$.
When $h \ge 2$, note there are $6$ state action pairs $(s_1,a)$, $(s_1,b)$, $(s_2,a)$, $(s_2,b)$, $(s_3,a)$, $(s_1,b)$.
With uniform exploration strategy, the underlying true regressor has the following form:\begin{align*}
B = \begin{pmatrix}
0.09 & 0.01 & 0 & 0 & \ldots & 0 \\
0 & 0 & 0.025 & 0 &\ldots & 0 \\
0 & 0 & 0.025 & 0 & \ldots & 0 \\
0.01 & 0.09 & 0 & 0 & \ldots & 0 \\
0 & 0 & 0.025 & 0 & \ldots & 0\\
0 &0 & 0.025 & 0 & \ldots & 0\\
\end{pmatrix}.
\end{align*} 
To see this if $x \sim E(s_1)$, \begin{align*}
	Bx = \begin{pmatrix}
	0.09 & 0.01 & 0 & 0 & \ldots & 0 \\
	0 & 0 & 0.025 & 0 &\ldots & 0 \\
	0 & 0 & 0.025 & 0 & \ldots & 0 \\
	0.01 & 0.09 & 0 & 0 & \ldots & 0 \\
	0 & 0 & 0.025 & 0 & \ldots & 0\\
	0 &0 & 0.025 & 0 & \ldots & 0\\
	\end{pmatrix} \begin{pmatrix}
	10\\
	0 \\
	0 \\
	? \\
	\ldots\\
	?
	\end{pmatrix} = \begin{pmatrix}
	0.9\\
	0 \\
	0 \\
	0.1 \\
	0 \\
	0 \\
	0
	\end{pmatrix} 
\end{align*} which is exactly $P(\cdot,\cdot|s_1)$.
We can check other conditional probability as well.

In this experiment, we test whether we can learn good $g_h$ and transition probability $\hat{P}$.
We sample some $\hat{g}_h$.

$\hat{g}_3$: \begin{verbatim}
0.0902    0.0096    0.0000    0.0025   -0.0009
0.0000    0.0000    0.0256    0.0057   -0.0009
0.0000    0.0000    0.0250    0.0044    0.0004
-0.0000   -0.0000    0.0243   -0.0075    0.0026
-0.0000   -0.0000    0.0251   -0.0026   -0.0021
0.0098    0.0904   -0.0000   -0.0025    0.0009
\end{verbatim}

$\hat{g}_7$: \begin{verbatim}
0.0000    0.0000    0.0252    0.0020    0.0037
0.0107    0.0913    0.0000    0.0021   -0.0017
-0.0000   -0.0000    0.0246   -0.0027   -0.0016
-0.0000    0.0000    0.0245    0.0059    0.0003
0.0893    0.0087   -0.0000   -0.0021    0.0017
-0.0000   -0.0000    0.0257   -0.0052   -0.0024
\end{verbatim}

$\hat{g}_{10}$: \begin{verbatim}
0.0000    0.0000    0.0250   -0.0046    0.0045
-0.0000   -0.0000    0.0250    0.0062   -0.0073
0.0890    0.0104   -0.0000    0.0015   -0.0019
0.0000   -0.0000    0.0246   -0.0061   -0.0010
-0.0000    0.0000    0.0254    0.0045    0.0039
0.0110    0.0896    0.0000   -0.0015    0.0019
\end{verbatim}

Note the order may not match because we don't observe the state directly, the order is based on we learned.

We also report the estimated transition probability.
For each state we report three matrix, each representing $P(\cdot|s,\cdot)$ for $s=s_1,s_2,s_3$.
Each row represents an action.

$\hat{P}_3:$
\begin{verbatim}
1     0     0
1     0     0

1.0000         0         0
0    0.9080    0.0920

0    0.0959    0.9041
1.0000         0         0
\end{verbatim}

$\hat{P}_7:$
\begin{verbatim}
1     0     0
1     0     0

0    0.9065    0.0935
1.0000         0         0

1.0000         0         0
0    0.0869    0.9131
\end{verbatim}

$\hat{P}_{10}:$
\begin{verbatim}
0     1     0
0     1     0

0    1.0000         0
0.0988         0    0.9012

0.8943         0    0.1057
0    1.0000         0
\end{verbatim}
